# Supplementary material for: Small-world topology of functional connectivity in randomly connected dynamical systems
Source: arXiv:1206.3963 ancillary file (2012-06-18)
Supplement: Supplementary file 1 [file SI.pdf]

# Supplemental Material
# ‘Small-world topology of functional connectivity in randomly connected dynamical system’

J. Hlinka and D. Hartman and M.Paluš

May 19, 2012

Summary of simulation results is visualized in the following figures.

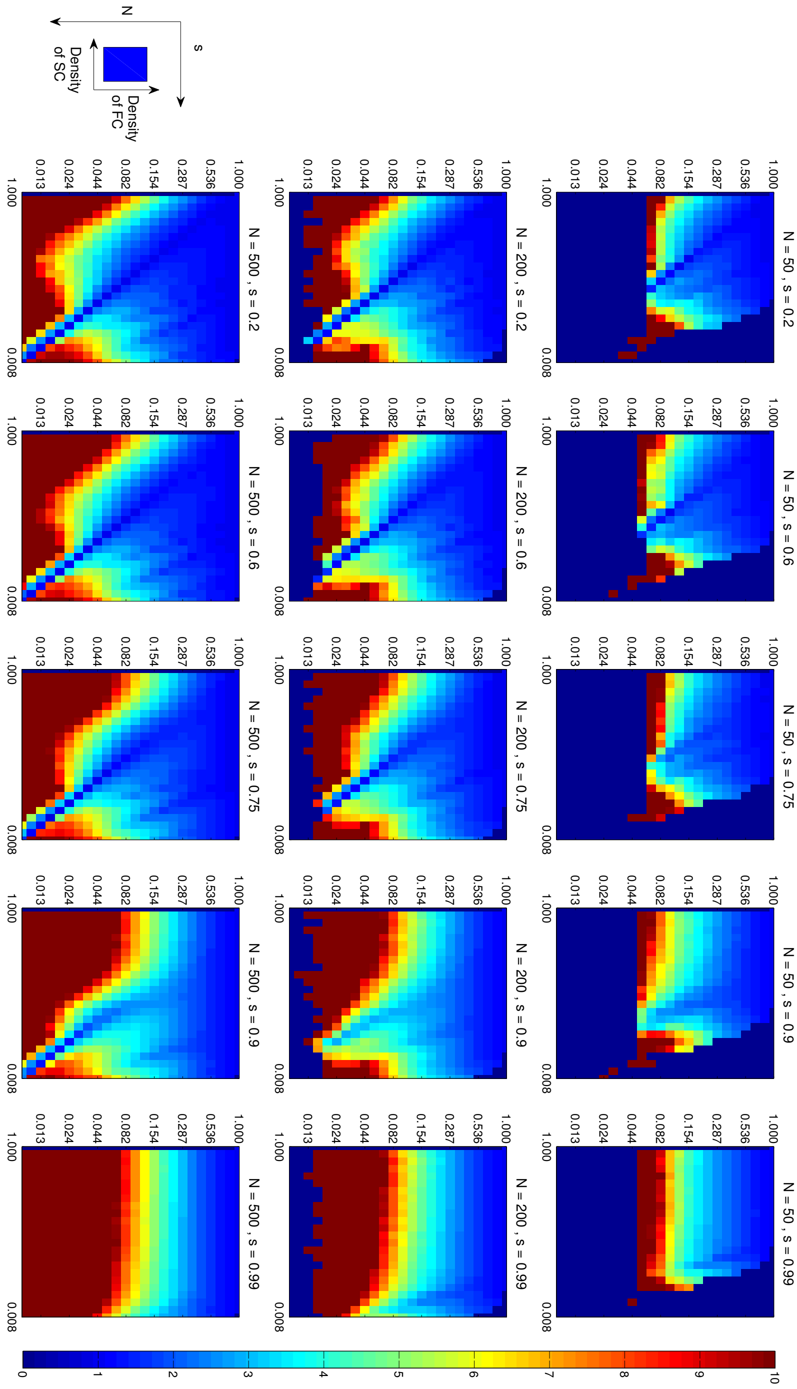


Figure 1: Average values of the small-world index $\sigma$ of the binarized functional connectivity $F$ generated by AR model with random connectivity matrix $S$. In most of the parameter space, $\sigma \gg 1$, suggesting small-world topology. The values markedly depend on the density of $S$ and $F$, less so on the values of $N$ and $s$. Other settings: $\alpha = 1$. In some parts of the parameter space, $\sigma$ was not well defined due to division by zero, mainly for small matrices ($N = 50$) and the values set plotted as zero (dark blue). Similarly there are missing values in the part of parameter space corresponding to very sparse $S$ matrices, as these generate only sparse $F$ matrices.

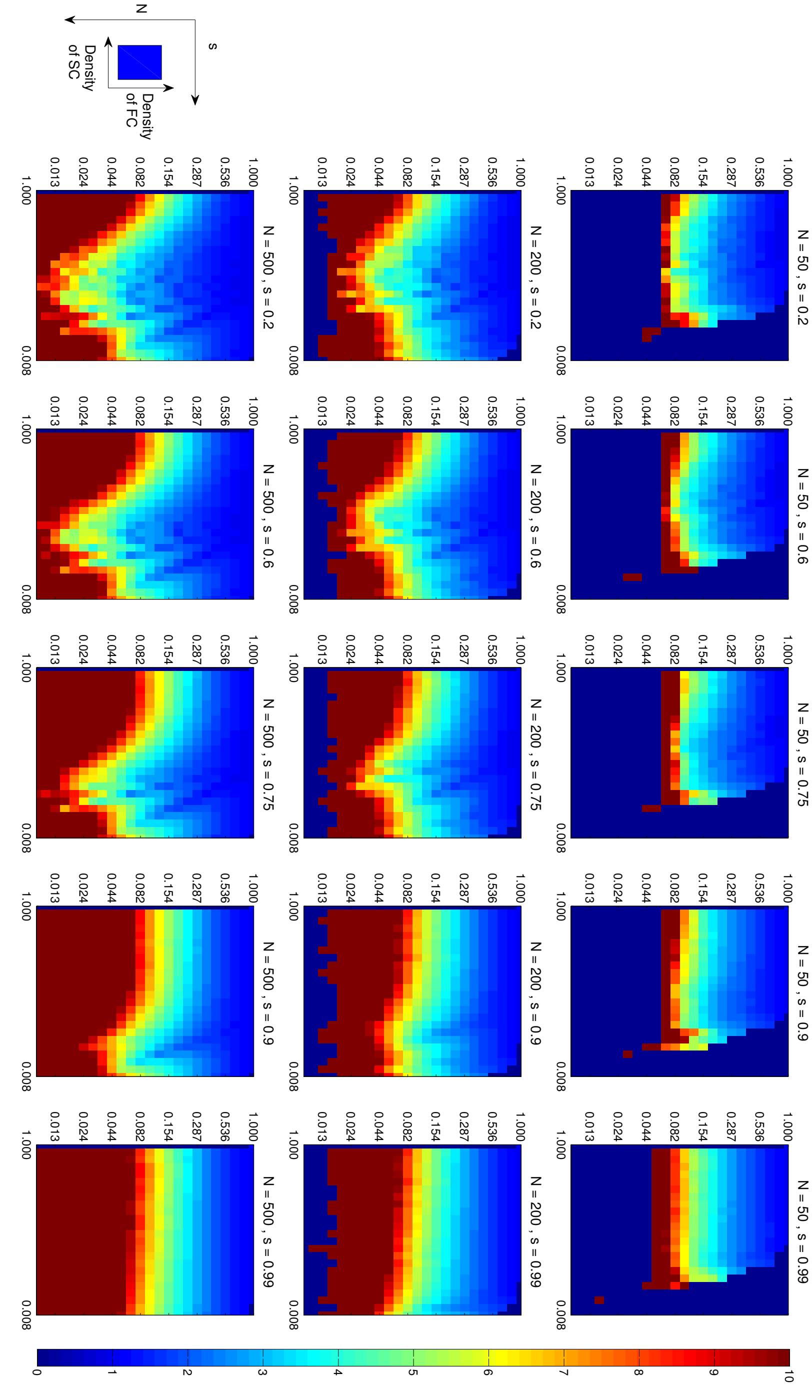


Figure 2: Average values of the small-world index $\sigma$. Visualization as in Figure 1, $\alpha = 0$.

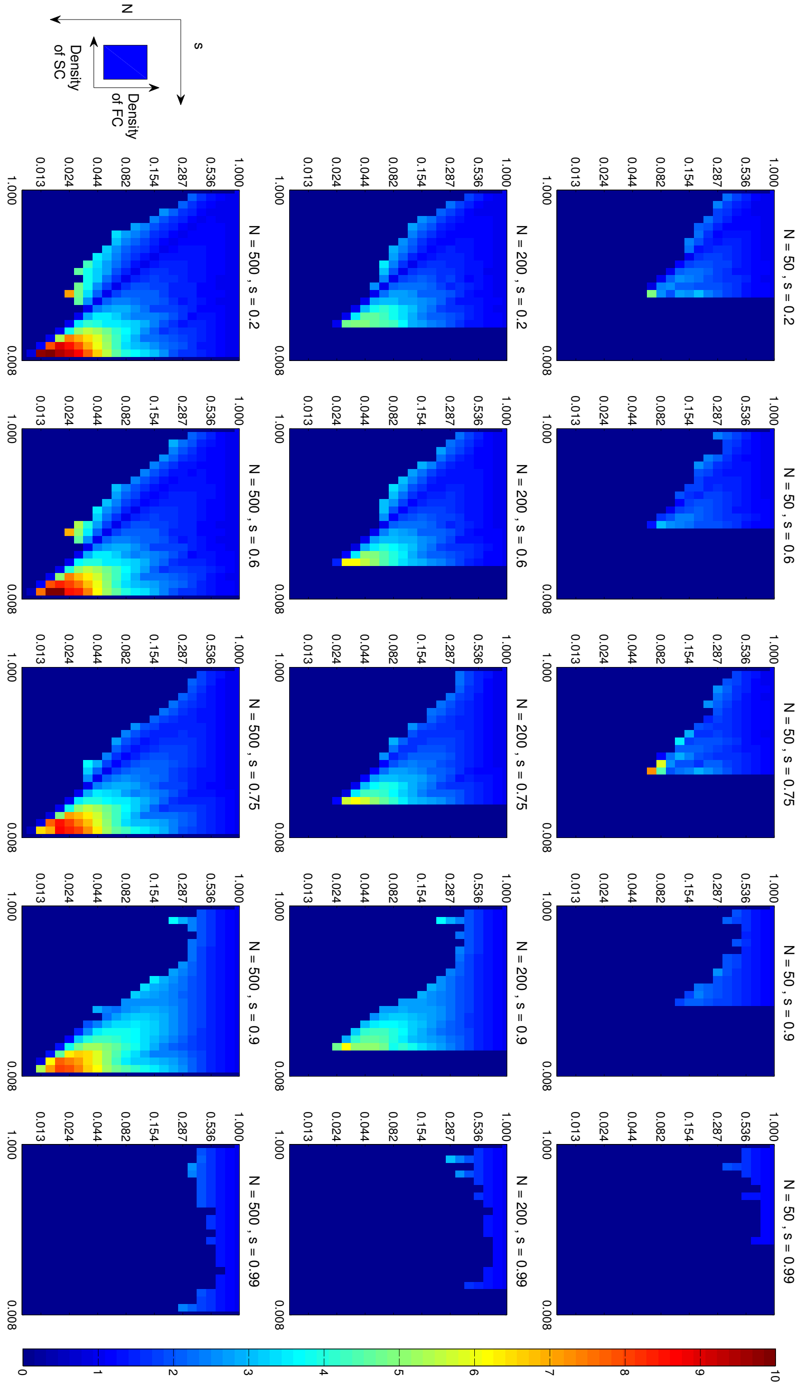


Figure 3: Average values of the small-world index $\sigma$, computed for connected (i.e. single component) graphs only. Visualization and settings as in Figure 1.

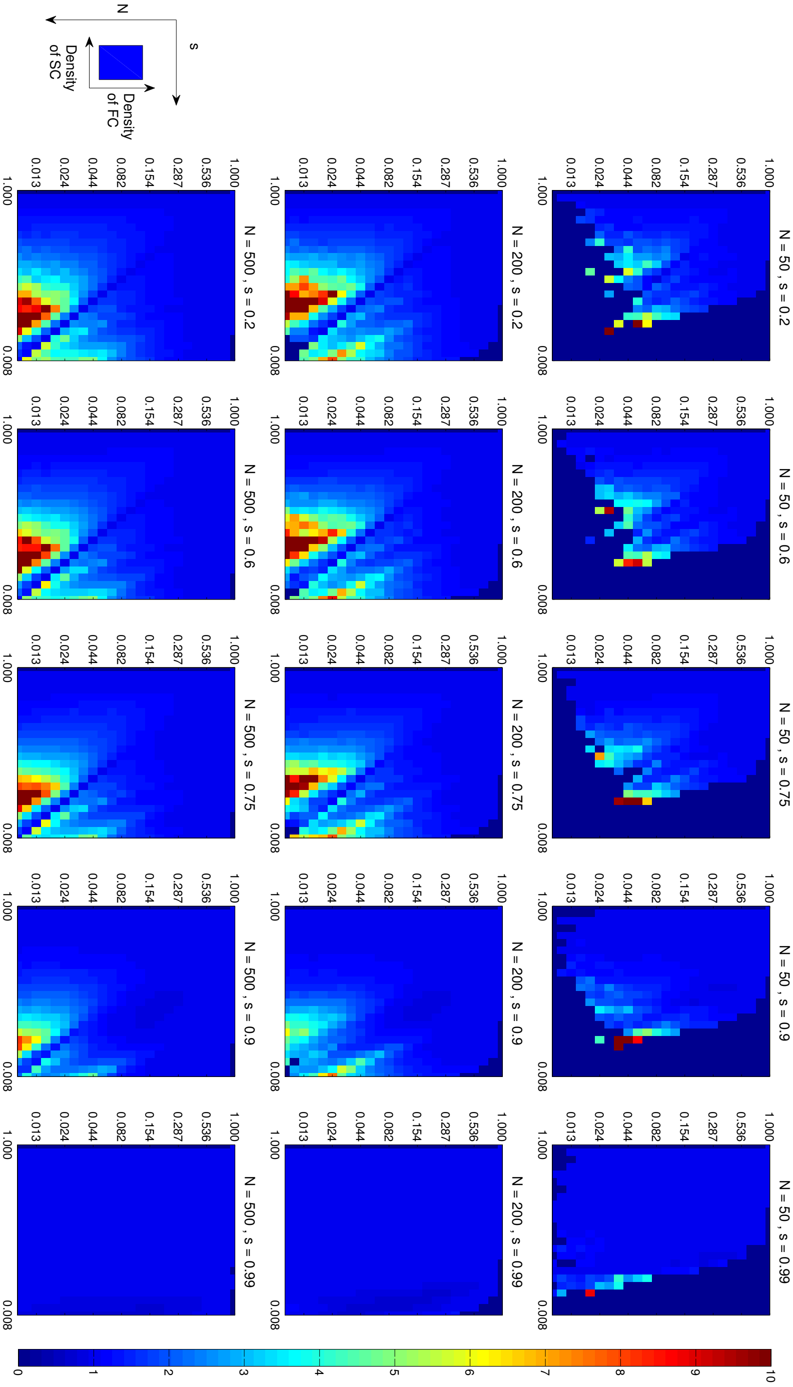


Figure 4: Average values of the small-world index $\sigma$ with the use of Maslov-Sneppen instead of Erdős-Rényi random graph model realizations as reference. Visualization and settings as in Figure 1.

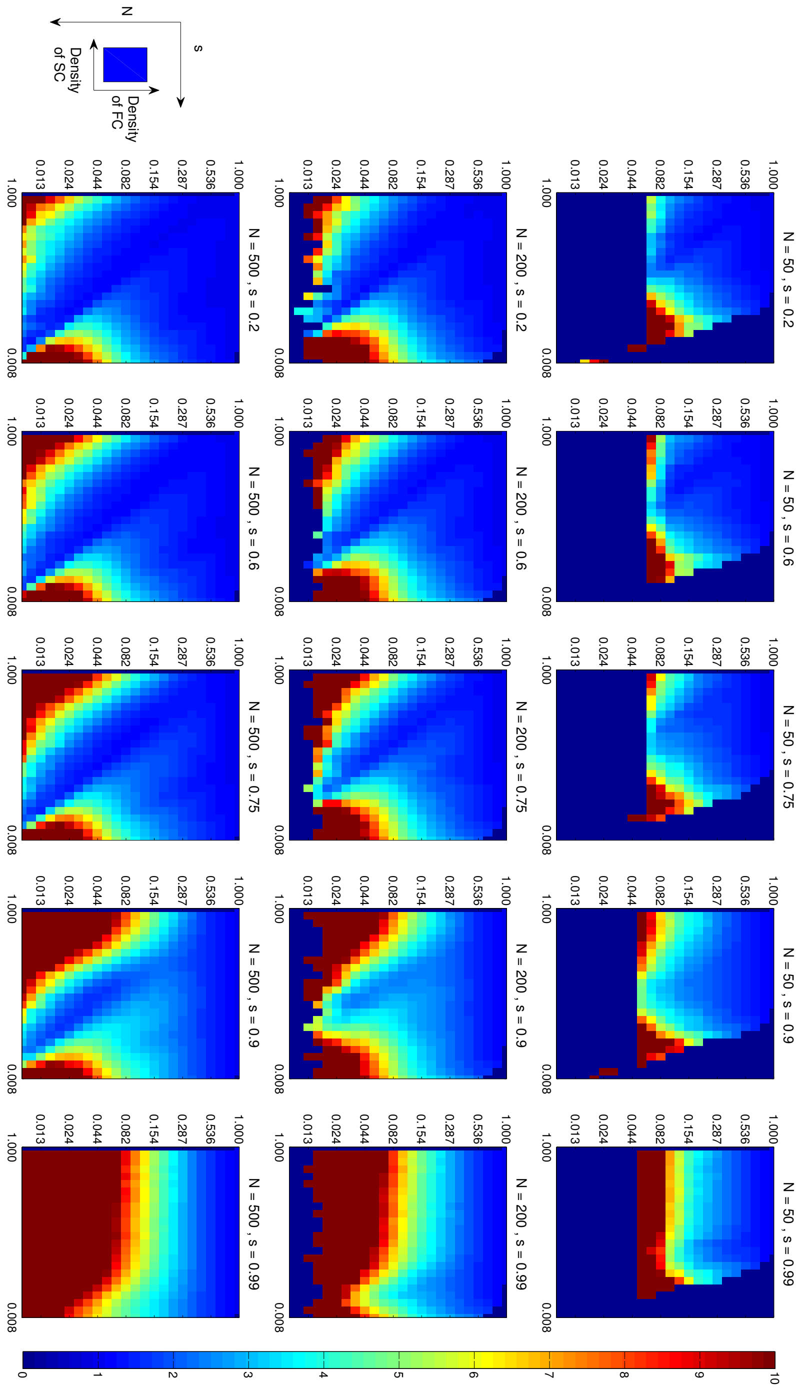


Figure 5: Average values of the small-world index $\sigma$ with the use of uniform (on interval $[0, 1]$) rather than binary value distribution for the underlying structural connectivity matrix $S$. Visualization and settings as in Figure 1.

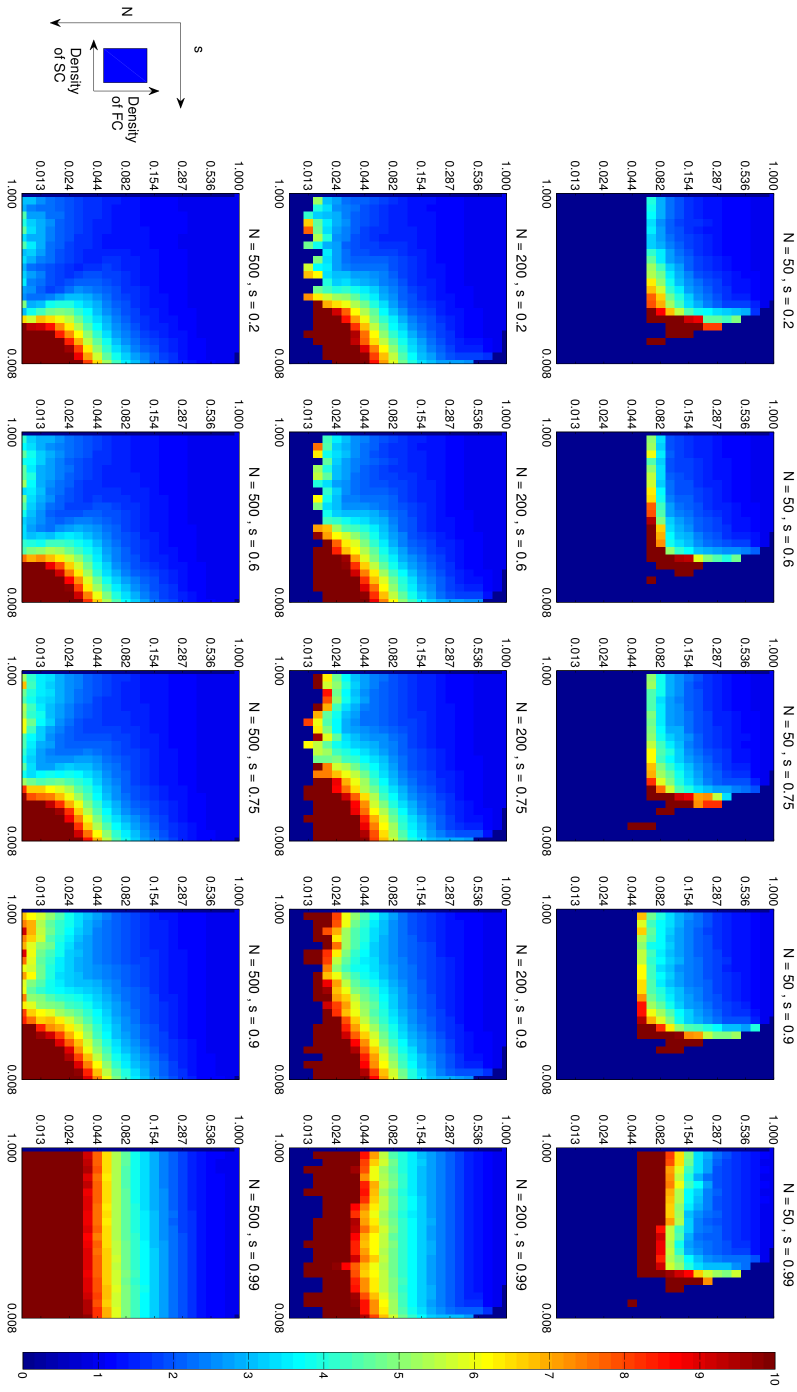


Figure 6: Average values of the small-world index $\sigma$ with the use of standard gaussian ($\mathbb{N}(0,1)$) rather than binary value distribution for the underlying structural connectivity matrix $S$. Visualization and settings as in Figure 1.
